# Supplementary material for: Double Mixture: Towards Continual Event Detection from Speech
Source: arXiv:2404.13289 source file (2024-10-28)
Supplement: Supplementary file 1 [file appendix.tex]

\appendix

\section{Experiment Setting}

\subsection{Datasets}

To evaluate the model's generalization ability in complex scenarios, we select some categories with a large number of samples from the above three speech data sets and reconstruct two data sets: Speech splicing and Speech overlaying. Speech splicing simulates the parallel occurrence of speech events by splicing two speech samples. In contrast, Speech overlaying simulates the overlap of speech events by superimposing speech samples, which poses a greater challenge to the model's recognition capabilities.

\input{table/dataset}

\subsection{Evaluation Metrics}
The evaluation criteria involve accessing a test set after the model completes a particular learning task $T_i$, followed by an assessment of the model's accuracy across all tasks within the curriculum, denoted by $R$.

\noindent \textbf{Average Accuracy.} To assess the overall performance across all learned tasks, we calculate incrementally after each newly introduced task:
\begin{equation}
    ACC=\frac{1}{T}\sum_{i=1}^{T}R_{T,i},
\end{equation}
where $R_{T,i}$ represents the performance metric on the $i$-th task after training on the $T$-th task.

\noindent \textbf{Forgetting Rate.} To understand whether learning new tasks has any detrimental effect on the model’s performance on previously learned tasks, we quantify the average loss in performance on earlier tasks, denoted as Forgetting Rate:
\begin{equation}
    Forgetting=\frac{1}{T}\sum_{i=1}^{T}R_{i,i}-R_{T,i},
\end{equation}
where $Forgetting$ spans the range $(-\infty, +\infty)$, with positive values indicating forgetting on the prior tasks, and negative ones suggesting performance improvement.

\subsection{Baselines}
We implement the following classic continual learning approaches: 
\begin{itemize}
    \item \textbf{Fine-tuning (FT).} Initially, we apply a sequential fine-tuning process to Whisper, utilizing cross-entropy loss to establish a foundational lower bound for CL performance. This method serves as a preliminary step to measure the model's adaptability across successive tasks.
    \item \textbf{Multi-task Learning (MTL).} In contrast, the MTL strategy involves simultaneous training on all available data, setting an upper bound. 
    \item \textbf{Experience Replay (ER)~\cite{rolnick2019experience}.} This rehearsal-based method leverages a data buffer to store and replay selected experiences from previous tasks. This method aims to mitigate the loss of prior knowledge by reintegrating past information during new task learning. 
    \item \textbf{Averaged Gradient Episodic Memory (A-GEM)~\cite{chaudhry2018efficient}.} A-GEM extends the concept of ER by enforcing inequality constraints on the loss function for past experiences. This ensures that while the model can improve on previous tasks, it does not accelerate the loss, thus offering a dynamic balance between retaining old knowledge and acquiring new information.
    \item \textbf{Elastic Weight Consolidation (EWC)~\cite{kirkpatrick2017overcoming}.} This regularization-based method quantifies the significance of model parameters through the Fisher Information Matrix. This matrix assesses the impact of each parameter on past task performance, enabling the model to apply a tailored quadratic penalty to the loss function during current task training, thereby preserving essential knowledge.
    \item \textbf{Learning without Forgetting (LwF)~\cite{li2017learning}.} This regularization-based method utilizes a dual-model architecture where a frozen copy of the model acts as a teacher for the current, active model (student). This configuration allows the student model to learn from both the new task and the teacher, enriching its learning trajectory without forsaking prior knowledge.
    \item \textbf{Piggyback (PB)~\cite{mallya2018piggyback}.} This architecture-based method introduces an innovative architectural adjustment that involves the application of binary masks derived from learnable weights onto the frozen parameters of a base model. 
    % This selective masking technique facilitates the model's adaptability to new tasks by reconfiguring its existing parameters.
    \item \textbf{Learning to Prompt (L2P)~\cite{wang2022learning}.} This method employs a collection of learnable vectors (prompts) that are dynamically integrated into a pre-trained model. This method allows for the customization of the model's responses to tasks, providing a flexible mechanism for task-specific adaptation.
\end{itemize}

\subsection{Implementation Details}
We train the models for 10 epochs per task using AdamW~\cite{loshchilov2017decoupled} with an initial learning rate of 0.0001, and we use a batch size is 16. After each epoch, the learning rate is reduced by 20\% if no validation performance improvement is observed. We clip the gradient L2 norm to 5 to enhance stability. We also freeze Whisper’s encoder and enable automatic mixed-precision to reduce memory consumption and speed up training. We use whisper-base\footnote{\url{https://huggingface.co/openai/whisper-base}} as the backbone and apply greedy decoding at inference. We retain 10\% of the data from each previous task, about 20 to 100 samples. The combination of speech in memory is different from the test set. All experiments are run on a single RTX 4090.
